# Supplementary material for: First measurement of the $CP$-violating phase in $B^0_s\to J/\psi(\to e^+e^-)\phi$ decays
Source: arXiv:2105.14738 source file (2021-12-08)
Supplement: Supplementary file 3 [file supplementary.tex]

\section{Supplementary material for LHCb-PAPER-2020-042}
\label{sec:Supplementary-App}

The supplementary material for LHCb-PAPER-2020-042 provides additional details of the analysis.
Fig.~\ref{fig:BDTresponse} and Table~\ref{tab:RankingBDT} present results of the BDT training.
In Fig.~\ref{fig:BsMassMCPeakBkg} the results of a simulation study for background contamination to signal region are presented.
Table~\ref{tab:FTperformance} shows details of the tagging performance.

\begin{figure}[!htb]
  \begin{center}
    \includegraphics[width=0.5\linewidth]{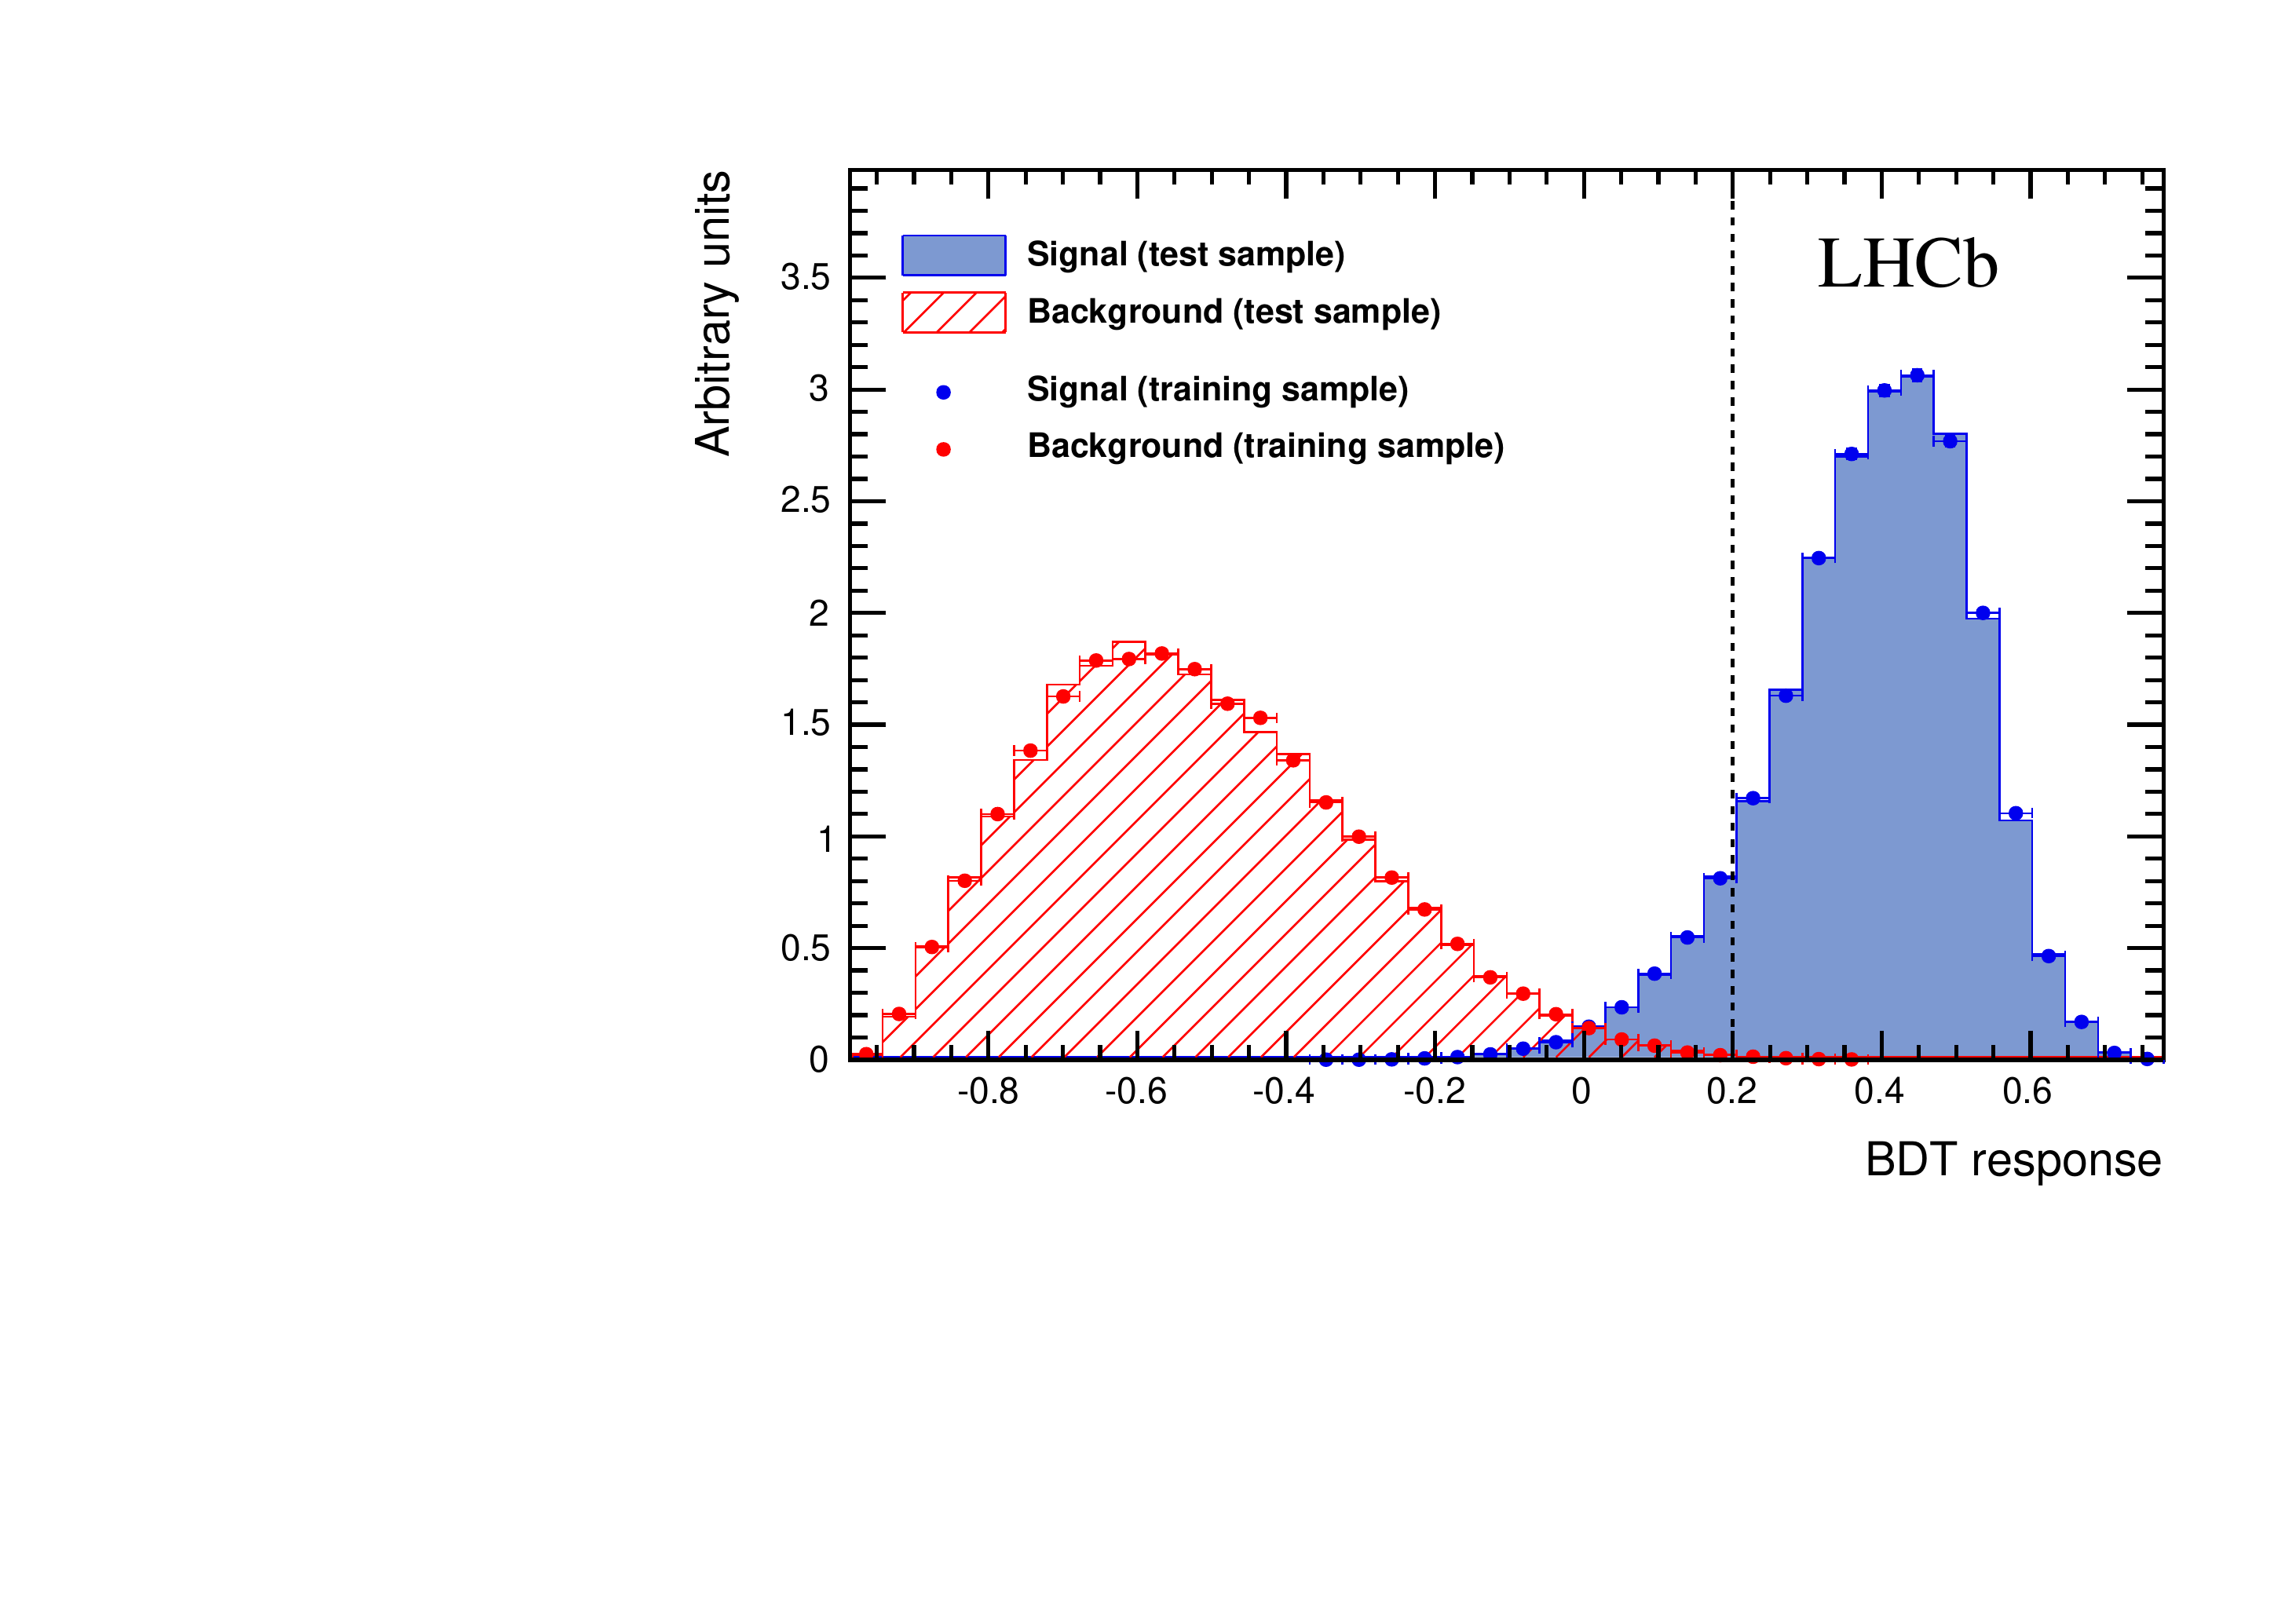}
%   \vspace*{-0.5cm}
  \end{center}
  \caption{
    \small %captions should be a little bit smaller than main text
    Distributions of the BDT variable for both training and test samples of \decay{\Bs}{\jpsi(}{\epem)\phiz} signal and background events. The signal samples are from simulation (blue) and the background samples derived from the same-sign data combination (red). The black dotted line indicates the chosen minimum BDT requirement.}
  \label{fig:BDTresponse}
\end{figure}

   \begin{table}[!htb]
  \caption{\small Variables used in the BDT selection: the transverse momenta of the \jpsi and \phiz candidates, \pt(\jpsi) and \pt(\phiz); the vertex \chisq of the \Bs candidate, \chisqvtx(\Bs); the \chisq of \Bs candidate kinematic fit with the \jpsi mass constrained to its PDG value, $\chisq_{\mathrm{DTF}}$(\Bs); the electron and kaon identification probabilities as provided mainly from the RICH and calorimeter systems, PIDe(\epm) and ProbNNK(\Kpm). The importance is evaluated as the total separation-gain that this variable had in the decision trees (weighted by the number of events)~\cite{Hocker:2007ht}.}
\begin{center} \begin{tabular}{cc}
    \toprule
   Variable & Importance  \\
    \midrule
  PIDe(\ep) & $0.18$ \\
  PIDe(\en) & $0.17$ \\
  log(ProbNNK)(\Kp) & $0.14$ \\
  log(ProbNNK)(\Km) & $0.13$ \\
  \pt(\jpsi) & $0.11$ \\
  \pt(\phiz) & $0.10$ \\
  log$(\chisq_{\mathrm{DTF}})(\Bs)$ & $0.09$ \\
  \chisqvtx(\Bs) & $0.08$ \\
  \bottomrule
    \end{tabular}\end{center}
\label{tab:RankingBDT}
\end{table}

\newpage
 \begin{figure}[!htb]
   \begin{center}
   \includegraphics[width=0.5\linewidth]{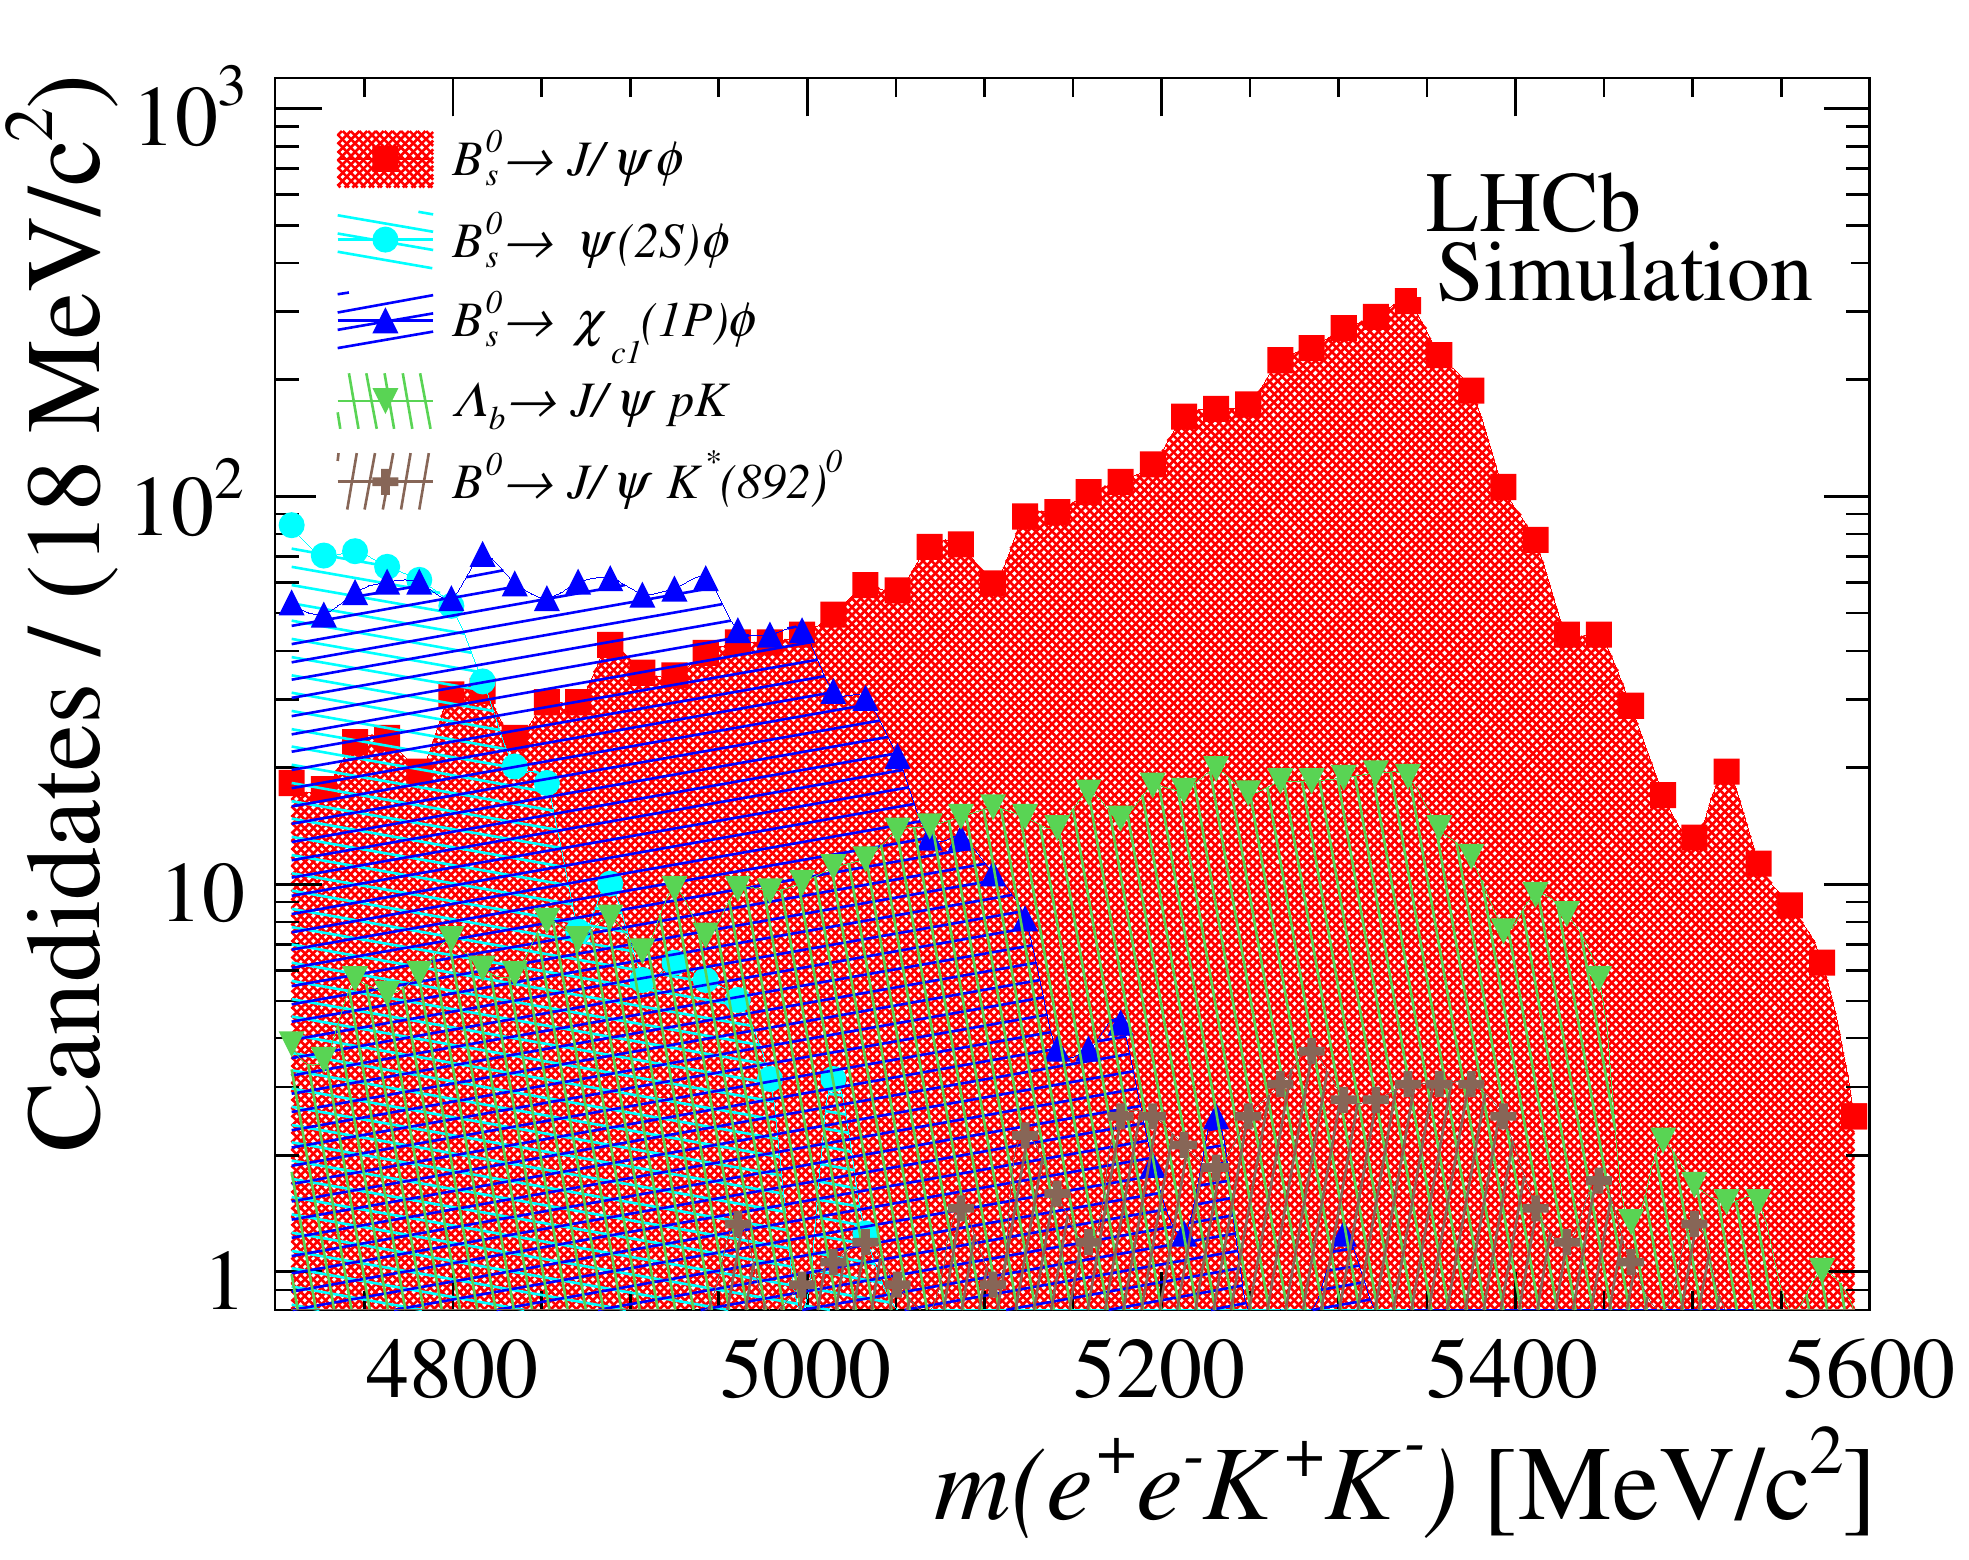}
   \end{center}
   \caption{
     \small 
     Distribution of the reconstructed mass of simulated \Bs candidates. The red area shows the signal \decay{\Bs}{\jpsi\phiz} candidates. The green and brown areas areas correspond to candidates selected from \decay{\Lb}{\jpsi p\Km} and \decay{\Bd}{\jpsi\Kstar(892)^0} decays, respectively, that are mis-reconstructed as \decay{\Bs}{\jpsi\phiz} due to proton and pion misidentification as kaon or due to partially random combinations with other tracks. The light blue and blue areas show the partially reconstructed background contribution from \decay{\Bs}{\psitwos\phiz} and \decay{\Bs}{\chicone(1P)\phiz} decays, respectively.}
   \label{fig:BsMassMCPeakBkg}
 \end{figure}

\begin{table}[!htb]
\caption{\small 
    Tagging efficiency $\varepsilon_{\mathrm{tag}}$, squared average tagging dilution $\mathcal{D}^{2}$ and tagging power $\varepsilon_{\mathrm{eff}}$ of the \decay{\Bs}{\jpsi\phiz} signal candidates for the data sample in the three tagging categories. The column ``Fraction'' reports the fraction of events in each category out of the all tagged events.}
\begin{center}\begin{tabular}{ccccc}
\toprule
Category & Fraction(\%)&$\varepsilon_{\mathrm{tag}}$(\%) & $\mathcal{D}^{2}$ & $\varepsilon_{\mathrm{eff}}$(\%)\\
\midrule
OS-only & $11.1$ &$10.72\pm0.73$ & $0.1157\pm0.0105$ & $1.24\pm0.09$ \\
SSK-only & $41.6$ &$40.20\pm1.14$ & $0.0279\pm0.0013$ & $1.12\pm0.04$ \\
OS\&SSK& $25.5$ &$24.70\pm1.01$ & $0.1097\pm0.0068$ & $2.71\pm0.13$ \\
\midrule
Total & $78.2$ & $75.62\pm1.69$& $0.0670\pm0.0028$ & $5.07\pm0.16$ \\
\bottomrule
\end{tabular}\end{center}
\label{tab:FTperformance}
\end{table}
